# Supplementary material for: Harpagon: Minimizing DNN Serving Cost via Efficient Dispatching, Scheduling and Splitting
Source: arXiv:2412.06161 source file (2024-12-09)
Supplement: Supplementary file 1 [file 07.appendix.tex]

\appendix
\section{Appendix}
% \subsection{Deriving Scheduling Results for \codesub{S}{1} to \codesub{S}{4}}
\subsection{\texorpdfstring{Deriving Scheduling Results for \codesub{S}{1} to \codesub{S}{4}}{Deriving Scheduling Results for S1 to S4}}
\label{appendix:deriving_scheduling}
% As discussed in \secref{sec:background}, for a workload of module \codesub{M}{3} from \tabref{tab:batch_example} with request rate of $\texttt{T}=198$ req/sec and latency SLO of $1.0$ sec, \tabref{tab:scheduling_example} shows the scheduling results and serving cost for scheduling methods \codesub{S}{1} to \codesub{S}{4}. We now provide a detailed analysis on how we derive them as follows.

We now provide a detailed analysis on how to derive the scheduling results and serving cost for scheduling method \codesub{S}{1} to \codesub{S}{4} in \tabref{tab:scheduling_example} for the workload of \codesub{M}{3} with request rate of $\texttt{T}=198$ req/sec and latency SLO of $1.0$ sec.

\parab{Result for \codesub{S}{1}.} As shown in \tabref{tab:scheduling_example}, scheduling method \codesub{S}{1} dispatches requests among machines with RR dispatch and assigns up to two configurations for each module. Under RR dispatch, the worst case latency $\codesub{L}{wc}=\texttt{2d}$ for batch size of $2$, $8$ and $32$ will be $0.2$, $0.5$ and $1.6$ sec respectively. To satisfy the latency objective of $1.0$ sec, \codesub{S}{1} can \textit{not} choose batch size of $32$ since its \codesub{L}{wc} violates the latency SLO. Instead, \codesub{S}{1} chooses batch size of $8$ as the majority configuration, and allocates $\lfloor \texttt{T}/\codesub{t}{maj}\rfloor=\lfloor 198/32\rfloor=6$ machines at batch size of $8$, leading to a majority workload of $192$ req/sec. For the residual workload of $198-192=6$ req/sec, \codesub{L}{wc} for batch size of $2$ and $8$ will be $0.1+2/6=0.43$ and $0.25+8/6=1.58$ sec. Similarly, to satisfy the latency SLO of $1.0$ sec, \codesub{S}{1} will choose batch size of $2$ for the residual workload.

Therefore, \codesub{S}{1} allocates $6$ machines at batch size of $8$ at full capacity for the majority workload of $192$ req/sec and one machine at batch size of $2$ at partial capacity of $6/20=0.3$ for the residual workload of $6$ req/sec, leading to a serving cost of $6+0.3=6.3$ machines as shown in \tabref{tab:scheduling_example}.

\parab{Result for \codesub{S}{2}.} Different from \codesub{S}{1}, scheduling method \codesub{S}{2} dispatches batched requests among machines with TC dispatch. Under TC dispatch, $\codesub{L}{wc}=\texttt{d}+\texttt{b}/\texttt{T}$ for batch size of $2$, $8$ and $32$ will be $0.11$, $0.29$ and $0.96$ sec, all of which can satisfy the latency objective of $1.0$ sec. \codesub{S}{2} can now choose batch size of $32$ as the majority configuration, which is infeasible for \codesub{S}{1} due to its low batch collection rate under RR dispatch. \codesub{S}{2} allocates $\lfloor \texttt{T}/\codesub{t}{maj}\rfloor=\lfloor 198/40\rfloor=4$ machines at batch size of $32$, leading to a majority workload of $160$ req/sec.

According to definition, \codesub{S}{2} only supports up to two configurations (\eg one for majority workload and the other for residual workload) per module. Therefore, for residual workload of $198-160=38$ req/sec, \codesub{S}{2} can only assign one configuration. \codesub{L}{wc} for batch size of $32$ will be $1.64$ sec, which violates the latency objective. For batch size of $8$, since the residual workload exceeds its module throughput ($38>32$), we will allocate two machines, whose equivalent batch collection rate is $38$ and $6$ req/sec respectively. The one with $6$ req/sec batch collection rate has \codesub{L}{wc} of $0.25+8/6=1.58$ sec, which again violates the latency objective. \codesub{S}{2} will then choose batch size of $2$ for the residual workload.

Therefore, \codesub{S}{2} allocates $4$ machines at batch size of $32$ at full capacity for the majority workload of $160$ req/sec, alongside one machine at batch size of $2$ at full capacity and one machine at batch size of $2$ at partial capacity of $(38-20)/20=0.9$, leading to a serving cost of $4+1+0.9=5.9$ machines.

\parab{Result for \codesub{S}{3}.} Different from \codesub{S}{2}, scheduling method \codesub{S}{3} has no limitation on the number of configurations for each module. Similar to \codesub{S}{2}, \codesub{S}{3} will also allocate $4$ machines at batch size of $32$ to deal with a majority workload of $160$ req/sec. For the residual workload of $38$ req/sec, since \codesub{S}{3} supports any number of configurations for each module, \codesub{S}{3} will allocate one machine at batch size of $8$ and one machine at batch size of $2$. Therefore, \codesub{S}{3} allocates $4$ machines at batch size of $32$ at full capacity for the majority workload of $160$ req/sec, alongside one machine at batch size of $8$ at full capacity and one machine at batch size of $2$ at partial capacity of $(38-32)/20=0.3$, leading to a serving cost of $4+1+0.3=5.3$ machines.

\parab{Result of \codesub{S}{4}.} Scheduling method \codesub{S}{4} adds dummy requests to increase the achieved througput for machines of the residual workload. Specifically, \codesub{S}{4} adds dummy request of $2$ req/sec to the original workload of $198$ req/sec , leading to a new workload of $200$ req/sec. Under the new workload, the worst case latency for batch size of $2$, $8$ and $32$ with TC dispatch will be $0.11$, $0.29$ and $0.96$ sec respectively. \codesub{S}{4} will allocate $5$ machines for the majority workload of $200$ req/sec, leaving a residual workload of $0$ req/sec. Therefore, \codesub{S}{4} allocates $5$ machines at batch size of $32$ at full capacity, leading to a serving cost of $5$ machines.

\subsection{Proof of \theoremref{theorem:leftover_workload}}
\label{appendix:leftover_proof}
\begin{proof}
We use proof of contradiction, where $\exists k \in \mathbb{K}, u_k=\sum_{j=k+1}^K n_jt_j \ge t_k$. For $u_k$, we define the total number of machine as $n_{\alpha}=\sum_{j=k+1}^K n_j$, the average unit price as $p_{\alpha}=\sum_{j=k+1}^K n_jp_j/n_{\alpha}$, and the average throughput as $t_{\alpha}=u_k/n_{\alpha}$. The total cost for $u_k$ is $C_0=\sum_{j=k+1}^K n_jp_j$. Since $u_k\ge t_k$, we allocate a new machine at $c_k$ to handle $t_k$ workload for higher throughput-cost. Depending on the worst case latency for the remaining $u_k-t_k$ workload, there will be two cases.
% We use proof of contradiction, where $\exists k \in \mathbb{M}, u_k=\sum_{j=k+1}^M n_jt_j \ge t_k$. For $u_k$, we define the average throughput as $t_p=\sum_{j=k+1}^M n_jt_j/\sum_{j=k+1}^M n_j$, the average number of machine as $n_p=u_k/t_p=\sum_{j=k+1}^M n_j$ and the average unit price as $c_p=\sum_{j=k+1}^M n_jc_j/\sum_{j=k+1}^M n_j$. Under the current cost-minimum configuration, the total cost for $u_k$ is $C_1=\sum_{j=k+1}^M n_jc_j=n_pc_p=c_p\frac{u_k}{t_p}$. Since $u_k\ge t_k$, we allocate a new machine at $c_k$ to handle $t_k$ amount of workload, and select new configuration for the remaining $u_k-t_k$ amount of workload. Depending on the worst case latency for the remaining $u_k-t_k$, there will be two cases.

In the first case, the original configuration for $u_k-t_k$ can still satisfy the latency constraint, then \sysname will switch $t_k$ amount of workload from its original configuration to $c_k$ for higher throughput-cost efficiency and keep $u_k-t_k$ workload unchanged. We define $T_1=\lfloor u_k/t_k\rfloor\cdot t_k$, then the new total cost for $u_k$ is $C_1=p_k\cdot\lfloor u_k/t_k\rfloor+p_{\alpha}\cdot(u_k-T_1)/t_{\alpha}$. We have $C_0-C_1=T_1(p_{\alpha}/t_{\alpha}-p_k/t_k)$. According to definition, $t_k/p_k>t_{\alpha}/p_{\alpha}$, so $C_0-C_1>0$. Namely, the cost-minimum assumption is violated.

% In the first case, configuration $c_k$ can satisfy the latency constraint, then we switch $u_k-t_k$ amount of workload to $c_k$. We define $T_1=\lfloor u_k/t_k\rfloor\cdot t_k$, then the new total cost for $u_k$ is $C_2=c_k\cdot\lfloor u_k/t_k\rfloor+c_p\cdot(u_k-T_1)/t_p$. We have $C_1-C_2=T_1(c_p/t_p-c_k/t_k)$. According to the definition, configurations are ordered by throughput-cost ratio, so $C_1-C_2>0$. Namely, using a new machine at $c_k$ can further reduce the cost, which violates the cost-minimum assumption.

% First, if a configuration of $t_p$ can satisfy the latency constraint, then using a new machine at $c_k$ will further reduce the cost, which violates the cost-minimum assumption. The intuition is that by switching the configuration from $t_p$ to $t_k$, $t_k$ amount of workload will run at a higher throughput-cost efficiency, while the remaining $t_u-t_k$ amount of workload will run at the original throughput-cost efficiency, leading to a lower total cost. Specifically, we define $T_1=\lfloor u_k/t_k\rfloor\cdot t_k$, then the new total cost for $u_k$ is $C_2=c_k\cdot\lfloor u_k/t_k\rfloor+c_p\cdot(u_k-T_1)/t_p=c_k\cdot T_1/c_k+c_p\cdot(u_k-T1)/t_p$. We have $C_1-C_2=c_p\cdot T_1/t_p-c_k\cdot T_1/t_k=T_1(c_p/t_p-c_k/t_k)$. According to the definition, the configuration is ordered by throughput-cost ratio, so $C_1-C_2>0$.

In the second case, the original configuration for $u_k-t_k$ can not satisfy the latency constraint, then \sysname will choose a new configuration $c_{\beta}$ to deal with the remaining $u_k-t_k$ workload to guarantee the latency SLO. Similarly, the new total cost for $u_k$ is $C_2=p_k\cdot \lfloor u_k/t_k\rfloor+p_{\beta}\cdot(u_k-T_1)/t_{\beta}$. We have $C_0-C_2=T_1(\frac{p_{\alpha}}{t_{\alpha}}-\frac{p_k}{t_k})-(u_k-T_1)(\frac{p_{\beta}}{t_{\beta}}-\frac{p_{\alpha}}{t_{\alpha}})$. According to definition, $T_1>u_k-T_1$, and for most modules, $\frac{p_{\alpha}}{t_{\alpha}}-\frac{p_k}{t_k} \approx \frac{p_{\beta}}{t_{\beta}}-\frac{p_{\alpha}}{t_{\alpha}}$, so $C_0-C2>0$. Namely, the cost-minimum assumption is violated.
\end{proof}
